# Supplementary material for: Drop the mask! GAMM-A Taxonomy for Graph Attributes Missing Mechanisms
Source: arXiv:2602.08407 source file (2026-02-09)
Supplement: Supplementary file 1 [file supplementary_material.pdf]

# Drop the mask! GAMM - A Taxonomy for Graph Attributes Missing Mechanisms
## Supplementary Material

Richard Serrano[1],[0009−0009−4946−896X],
Baptiste Jeudy[1][0009−0000−8126−2608],
Charlotte Laclau[2][0000−0002−7389−3191], and
Christine Largeron[1][0000−0003−1059−4095]

[1] Laboratoire Hubert Curien, Saint-Étienne 42000, France
{richard.serrano,baptiste.jeudy,christine.largeron}@univ-st-etienne.fr
[2] Télécom Paris, Institut Polytechnique de Paris, France
charlotte.laclau@telecom-paris.fr

Code : github.com/RichardSrn/GAMM

## A Experimental Protocol Details

This section provides supplementary details regarding the experimental setup, including comprehensive descriptions of the datasets used, the parameters for the missingness mechanisms, and a summary of notations.

### A.1 Datasets Description

Here we provide a more detailed description of the datasets used in our experiments.

First, table 1 offers a summary of the datasets. $H_{adj}$ represents the homophily of the networks, hence divided in 3 categories : (i) Homophilic when $H_{adj} > 0.5$, (ii) Neutral when $-0.1 < H_{adj} < 0.1$, and (iii) Heterophilic when $H_{adj} < -0.15$.

PLANETOID *datasets* (Cora, CiteSeer, PubMed) [5] represent homophilic networks with strong assortativity, featuring large-scale citation networks (2708, 3327, and 19717 nodes, respectively). They contain binary bag-of-words features (Cora, CiteSeer) or Word2Vec embeddings (PubMed) with high dimensionality (1433, 3703, and 500 features), and exhibit sparse connectivity patterns typical of citation networks.

WIKIPEDIA-*based graphs* Chameleon and Squirrel datasets, both extracted from Wikipedia [3], model article-level topics within a hyperlinked network. These medium-sized graphs feature 2277 and 5201 nodes, high-dimensional attributes, and a moderate level of homophily, making them applicable for testing nuanced structural dependencies in imputation tasks. On the other hand, the Actor

**Table 1.** Benchmark datasets, categorized by their adjusted homophily ($H_{adj}$).

| | Dataset | #Nodes | #Edges | #Classes | Features | $H_{adj}$ |
|---|---|---|---|---|---|---|
| Homophilic | Cora | 2708 | 5278 | 7 | $\{0,1\}^{1433}$ | 0.768 |
| | CiteSeer | 3327 | 4552 | 6 | $\{0,1\}^{3702}$ | 0.678 |
| Neutral | PubMed | 19717 | 44324 | 3 | $[0,2]^{500}$ | 0.693 |
| | Chameleon | 2277 | 18050 | 5 | $\{0,1\}^{2325}$ | 0.042 |
| | Squirrel | 5201 | 108536 | 5 | $\{0,1\}^{2089}$ | 0.030 |
| | Minesweeper | 10000 | 39402 | 2 | $\{0,1\}^{7}$ | 0.009 |
| | Actor | 7600 | 15009 | 5 | $\{0,1\}^{932}$ | 0.007 |
| | Roman-empire | 22662 | 32927 | 18 | $[0,1]^{300}$ | -0.045 |
| Heterophilic | Tolokers | 11758 | 519000 | 2 | $[0,1]^{10}$ | -0.188 |
| | Wisconsin | 251 | 257 | 5 | $\{0,1\}^{1702}$ | -0.189 |
| | Cornell | 183 | 149 | 5 | $\{0,1\}^{1702}$ | -0.219 |
| | Texas | 183 | 162 | 5 | $\{0,1\}^{1702}$ | -0.425 |

dataset, representing a social network in filmmaking [4], includes 7600 nodes characterized by moderate homophily, capturing dynamics where relationships occur across distinct groups in non-assortative environments.

HETEROPHILOUS *graph datasets* (Minesweeper, Roman-Empire, Tolokers) [2] represent very heterophilic networks with strong disassortative patterns. Their categorical features show low homophily ratios and present unique challenges for Graph Neural Networks. These medium-to-large-sized networks exhibit topological features that provide new opportunities to explore structural missingness, similar to the added datasets.

WEBKB *datasets* (Cornell, Texas, Wisconsin) [1] are moderately heterophilic networks where connected nodes often belong to different classes. These small webpage networks (183, 182, and 251 nodes respectively) use binary bag-of-words features with high dimensionality (1703) and display structural patterns representative of academic webpage link relationships between faculty, student, course, and project pages.

### A.2 Parameters for Missingness Mechanisms

The parameters used in the mechanisms for missingness mask generation are detailed in Table 2. The scaling parameters $\omega_k$ control the strength and the direction of the dependency of the missingness on the corresponding variables, while the bias terms $b_k$ are calibrated to ensure that the overall proportion of missing values matches the target rate $p_{\text{miss}}$.

The calibration of the bias terms $b_k$ is such that the expected missingness rate across all entries, $\mathbb{E}[\sigma(\cdot + b_k)]$, equals the target $p_{\text{miss}}$.

**Table 2.** Parameters for Missingness Mechanisms

| Parameter | Description | Default Value |
|---|---|---|
| $p_{\text{miss}}$ | Target missing rate | $\{20\%, 50\%, 80\%\}$ |
| $h$ | hop-distance | 1 |
| $\omega_1, \dots, \omega_5$ | Scaling parameters | 1 |
| $b_1, \dots, b_5$ | Bias terms | Calibrated |

### A.3 Notations

Table 3 provides a summary of the key notations used throughout the paper to describe the graph, features, and missingness components.

**Table 3.** Summary of Notations

| Symbol | Description |
|---|---|
| $G = (\mathcal{V}, \mathcal{E}, F)$ | Undirected attributed graph |
| $\mathcal{V}$ | Set of $n$ nodes |
| $\mathcal{E}$ | Set of edges |
| $F \in \mathbb{R}^{n \times d}$ | Node feature matrix |
| $F_{i\cdot} \in \mathbb{R}^d$ | Feature vector of node $v_i$ |
| $\Omega \in \{0,1\}^{n \times d}$ | Missingness mask (1 = observed) |
| $F^{(\text{OBS})}$ | Submatrix of $F$ with observed columns |
| $F^{(\text{MIS})}$ | Submatrix of $F$ with missing values |
| $\mathcal{N}_h(v_i)$ | Set of $h$-hop neighbors of node $v_i$ |
| $\text{dist}(v_i, v_j)$ | Geodesic distance between $v_i, v_j$ |
| $\mathfrak{S}(v_i)$ | Structural properties of node $v_i$ |
| $\mathfrak{S}_h(v_i)$ | Structural properties of $v_i$ś neighbors |
| $\mathfrak{N}_i^{(\text{OBS})}(h)$ | Observed features of $v_i$ś neighbors |
| $\mathfrak{N}_i^{(\text{MIS})}(h)$ | Missing features of $v_i$ś neighbors |

### A.4 Practical interpretation of $g(\cdot)$:

- **MCAR**: The probability of missingness is a constant $p_{\text{miss}}$, entirely independent of any data.
- **Attribute-based (A-MAR & A-MNAR)**: Missingness depends on the node's own features.
  - For **A-MAR**, the formula $g(F_{i\cdot}^{(\text{OBS})})$ shows that the probability depends on the *observed* features of the node. By setting $\omega_1$ to be positive or negative, we can make missingness more likely for nodes with high or low observed feature values, respectively.
  - For **A-MNAR**, missingness depends on the *values of the node that would be missing*, $F_{ij}^{(\text{MIS})}$. The term $\omega_2 \cdot F_{ij}^{(\text{MIS})}$ directly models this dependency.

– **Structure-based (S-MAR)**: Missingness is determined by a node's structural properties. The function uses the node's degree as input. By setting to be negative, for example, we model a scenario where nodes with a lower degree (more isolated nodes) are more likely to have missing attributes.
– **Neighbor-based (N-MAR & N-MNAR)**: Missingness is influenced by the attributes of a node's neighbors within an -hop neighborhood.
  • For **N-MAR**, the input $\mathfrak{N}_i^{(\text{OBS})}(h)$ is an aggregation (e.g., mean) of the *observed* features of a node's neighbors.
  • For **N-MNAR**, the input $\mathfrak{N}_i^{(\text{MIS})}(h)$ is an aggregation of the neighbors' features that are themselves subject to missingness, creating a more complex dependency.

These mechanisms allow us to explore two critical axes: the **information source** (node's own attributes, structure, or neighbors' attributes) and the **observability** (dependency on observed vs. unobserved data), providing a comprehensive framework for evaluating imputation methods.

## B Toy Example Details

The main paper uses a toy example in Figure 1 to illustrate the different missingness mechanisms. This section provides the underlying data for that example and a more detailed explanation.

*Scenario Description* The example depicts a corporate email network with 10 employees, where edges represent email exchanges. Node position reflects their *Hierarchy*: senior executives appear at the top, while junior employees are at the bottom. This spatial arrangement highlights how missingness correlates with attributes and network position. The attributes for each node are provided in Table 4.

**Table 4.** Node attributes for the example graph structure, linked to the mechanisms visualized in Figure 1 of the main paper.

| ID | Hierarchy | Age | Experience | Salary (k$) |
|---|---|---|---|---|
| E0 | 3 | 70 | 45 | 250 |
| E1 | 2 | 52 | 32 | 140 |
| E2 | 2 | 54 | 33 | 150 |
| E3 | 1 | 35 | 25 | 120 |
| E4 | 1 | 32 | 19 | 110 |
| E5 | 1 | 34 | 17 | 115 |
| E6 | 0 | 24 | 1 | 50 |
| E7 | 0 | 25 | 3 | 45 |
| E8 | 0 | 21 | 2 | 35 |
| E9 | 0 | 22 | 4 | 60 |

**Table 5.** Percentage degradation in MAE of N-MAR over A-MAR ($p_{\text{miss}} = 20\%$) across various datasets homophily. Negative results indicate deterioration in MAE with masking by the neighborhood-dependent (N-) mechanism compared to the attribute-dependent (A-) mechanism. An asterisk (*) indicates statistical significance ($p < 0.05$).

a) HOMOPHILIC datasets

| Imputer | CiteSeer | Cora | PubMed |
|---|---|---|---|
| Tabular_Avg | -0.0% | +1.7% | +0.4% |
| FP | -0.9% | +1.2% | +0.8% |
| GRIOT | -1.5% | -5.3% | +1.4% |
| Graph_1hop | -0.7% | +2.2% | +0.4% |
| OT-tab | +0.1% | +0.2% | -0.1% |
| PCFI | -5.7% | -0.4% | +2.3% |

b) HETEROPHILIC datasets

| Imputer | Tolokers | Cornell | Texas | Wisconsin |
|---|---|---|---|---|
| Tabular_Avg | -14.0%* | -0.7% | -1.7% | +0.4% |
| FP | -7.2%* | -3.4% | -5.6% | -3.7% |
| GRIOT | +0.0% | +2.1% | +7.1% | +11.2% |
| Graph_1hop | -12.6%* | +0.3% | +0.1% | +0.0% |
| OT-tab | -10.2%* | -1.7% | -0.2% | +0.9% |
| PCFI | -12.8%* | +7.2% | +4.6% | -5.2% |

c) NEUTRAL datasets

| Imputer | Actor | Chameleon | Squirrel | Minesweeper | Roman-empire |
|---|---|---|---|---|---|
| Tabular_Avg | +5.5% | -0.2% | +2.5% | -4.5% | -0.6% |
| FP | +5.9% | -0.4% | +2.7% | -2.8% | -0.4% |
| GRIOT | +1.5% | +0.1% | -0.4% | -0.0% | +0.7% |
| Graph_1hop | +0.6% | -0.3% | +1.9% | -0.9% | -0.5% |
| OT-tab | +0.1% | -0.2% | -0.0% | +8.3% | +0.0% |
| PCFI | -0.6% | -13.3%* | -8.1% | -1.9% | -0.9% |

## C Detailed Experimental Results

This section provides the complete and granular results of our experiments. We present the difference in Mean Absolute Error (MAE) between attribute-based (A-) and neighborhood-based (N-) mechanisms, as well as a comprehensive statistical summary.

### C.1 Difference in MAE: A-MAR vs. N-MAR

Tables 5, and 6 show the difference in MAE between the A-MAR and N-MAR mechanisms for a missing rate of 20%, and 50% respectively.

### C.2 Difference in MAE: A-MNAR vs. N-MNAR

Tables 7, 8, and 9 shows the difference in MAE between the A-MNAR and N-MNAR mechanisms for a missing rate of 20%, 50% and 80% respectively.

**Table 6.** Percentage degradation in MAE of N-MAR over A-MAR ($p_{\text{miss}} = 50\%$) across various datasets homophily. Negative results indicate deterioration in MAE with masking by the neighborhood-dependent (N-) mechanism compared to the attribute-dependent (A-) mechanism. An asterisk (*) indicates statistical significance ($p < 0.05$).

a) HOMOPHILIC datasets

| Imputer | CiteSeer | Cora | PubMed |
|---|---|---|---|
| Tabular_Avg | +0.2% | +1.6% | +1.3% |
| FP | -0.3% | +1.5% | +1.5% |
| GRIOT | +8.4% | -3.5% | -6.6% |
| Graph_1hop | -0.7% | +2.1% | +1.4% |
| OT-tab | +0.1% | +0.4% | +0.1% |
| PCFI | -25.8% | -5.5% | +5.1% |

b) HETEROPHILIC datasets

| Imputer | Tolokers | Cornell | Texas | Wisconsin |
|---|---|---|---|---|
| Tabular_Avg | -15.0%* | -0.4% | -3.0% | -0.1% |
| FP | -5.4% | -4.5% | +0.9% | -11.1% |
| GRIOT | +3.0% | -11.6% | -4.8% | +12.8% |
| Graph_1hop | -11.2%* | -1.1% | -0.7% | -0.6% |
| OT-tab | -9.7%* | -0.2% | -1.0% | +0.2% |
| PCFI | -11.5%* | -0.4% | +8.5% | +9.4% |

**Table 7.** Percentage degradation in MAE of N-MNAR over A-MNAR ($p_{\text{miss}} = 20\%$) across various datasets homophily. Negative results indicate deterioration in MAE with masking by the neighborhood-dependent (N-) mechanism compared to the attribute-dependent (A-) mechanism. An asterisk (*) indicates statistical significance ($p < 0.05$).

a) HOMOPHILIC datasets

| Imputer | CiteSeer | Cora | PubMed |
|---|---|---|---|
| Tabular_Avg | -50.6%* | -48.7%* | -9.1%* |
| FP | -72.9%* | -68.9%* | -15.5%* |
| GRIOT | -12.5% | -17.1%* | -5.1%* |
| Graph_1hop | -70.1%* | -64.4%* | -12.8%* |
| OT-tab | -10.3%* | -14.0%* | -2.1%* |
| PCFI | -55.6%* | -55.5%* | -13.0%* |

b) HETEROPHILIC datasets

| Imputer | Tolokers | Cornell | Texas | Wisconsin |
|---|---|---|---|---|
| Tabular_Avg | -9.0%* | -47.5%* | -46.5%* | -47.2%* |
| FP | -35.3%* | -46.1%* | -67.7%* | -54.4% |
| GRIOT | +0.9% | -77.1%* | -72.3%* | -72.4%* |
| Graph_1hop | -5.0%* | -53.1%* | -62.5%* | -54.3%* |
| OT-tab | -7.6%* | -30.8%* | -25.5%* | -31.2%* |
| PCFI | -4.0%* | -49.4%* | -38.3%* | -48.9%* |

c) NEUTRAL datasets

| Imputer | Actor | Chameleon | Squirrel | Minesweeper | Roman-empire |
|---|---|---|---|---|---|
| Tabular_Avg | -53.1%* | -38.8%* | -34.5%* | -23.1%* | +11.8%* |
| FP | -73.3%* | -86.8%* | -78.6%* | -27.4%* | -0.6% |
| GRIOT | -14.3%* | -11.2% | -14.1% | -0.0%* | +3.3%* |
| Graph_1hop | -63.5%* | -38.8%* | -36.0%* | -26.4%* | +6.2%* |
| OT-tab | -6.4%* | -6.2%* | -7.8%* | -20.1%* | +3.1%* |
| PCFI | -51.6%* | -17.2%* | -17.4%* | -25.5%* | +6.5%* |

**Table 8.** Percentage degradation in MAE of N-MNAR over A-MNAR ($p_{\text{miss}} = 50\%$) across various datasets homophily. Negative results indicate deterioration in MAE with masking by the neighborhood-dependent (N-) mechanism compared to the attribute-dependent (A-) mechanism. An asterisk (*) indicates statistical significance ($p < 0.05$).

a) HOMOPHILIC datasets

| Imputer | CiteSeer | Cora | PubMed |
|---|---|---|---|
| Tabular_Avg | -5.5%* | -6.8%* | -2.9%* |
| FP | -25.5%* | -24.3%* | -11.0%* |
| GRIOT | +0.4% | -5.9% | +22.8%* |
| Graph_1hop | -17.3%* | -17.6%* | -5.2%* |
| OT-tab | -8.0%* | -11.3%* | -2.1%* |
| PCFI | +28.7%* | +8.4% | -2.3% |

b) HETEROPHILIC datasets

| Imputer | Tolokers | Cornell | Texas | Wisconsin |
|---|---|---|---|---|
| Tabular_Avg | -34.8%* | -36.1%* | -30.1%* | -32.0%* |
| FP | -38.9%* | -70.4%* | -25.7% | -0.8% |
| GRIOT | -1.3%* | -110.3%* | -99.6%* | -52.2%* |
| Graph_1hop | -32.1%* | -37.8%* | -42.5%* | -39.3%* |
| OT-tab | -29.4%* | -35.1%* | -27.9%* | -33.8%* |
| PCFI | -32.5%* | -29.6%* | +14.2% | +6.3% |

**Table 9.** Percentage degradation in MAE of N-MNAR over A-MNAR ($p_{\text{miss}} = 80\%$) across various datasets homophily. Negative results indicate deterioration in MAE with masking by the neighborhood-dependent (N-) mechanism compared to the attribute-dependent (A-) mechanism. An asterisk (*) indicates statistical significance ($p < 0.05$).

a) HOMOPHILIC datasets

| Imputer | CiteSeer | Cora | PubMed |
|---|---|---|---|
| Tabular_Avg | +33.7%* | +32.5%* | +15.8%* |
| FP | +18.6%* | +20.1%* | +2.0%* |
| GRIOT | +41.1% | +10.1% | -1.5% |
| Graph_1hop | +29.9%* | +29.5%* | +14.7%* |
| OT-tab | -1.3%* | -1.9%* | -1.5%* |
| PCFI | +77.1%* | +55.5%* | +28.1%* |

b) HETEROPHILIC datasets

| Imputer | Tolokers | Cornell | Texas | Wisconsin |
|---|---|---|---|---|
| Tabular_Avg | -134.2%* | +5.8% | +4.5% | +7.6% |
| FP | -75.7%* | -26.0%* | -5.8% | +12.3% |
| GRIOT | +0.9%* | -21.3%* | -20.7%* | -17.8% |
| Graph_1hop | -160.0%* | +3.5% | +1.1% | +5.9% |
| OT-tab | -122.2%* | -9.4%* | -9.7%* | -9.9%* |
| PCFI | -157.3%* | -12.7% | +30.1%* | +36.6%* |

### C.3 Overall Statistical Summary

Table 10 provides a detailed summary of the statistical outcomes across all 2,304 experiments, categorized by the level of homophily in the datasets. This table expands on the summary provided in the main paper.

**Table 10.** Percentage Summary of Statistical Outcomes by Dataset Homophily. Total: 100% = 2,304 experiments.

| Category | Type | Sign. Degradation | No Sign. Change | Sign. Improvement | Total Tests |
|---|---|---|---|---|---|
| **Homophilic** | MAR | 3.2% | 9.0% | 1.5% | **13.7%** |
| | MNAR | 10.0% | 2.1% | 4.3% | **16.4%** |
| **Neutral** | MAR | 0.9% | 9.7% | 0.5% | **11.1%** |
| | MNAR | 11.9% | 3.2% | 3.5% | **18.6%** |
| **Heterophilic** | MAR | 3.8% | 13.5% | 0.9% | **18.3%** |
| | MNAR | 16.7% | 4.4% | 0.8% | **21.9%** |
| **Total** | | **46.6%** | **42.0%** | **11.4%** | **100.0%** |

## References

1. Craven, M., DiPasquo, D., Freitag, D., McCallum, A., Mitchell, T., Nigam, K., Slattery, S.: Learning to extract symbolic knowledge from the World Wide Web. AAAI/IAAI **3**(3.6), 2 (1998)
2. Platonov, O., Kuznedelev, D., Diskin, M., Babenko, A., Prokhorenkova, L.: A critical look at the evaluation of gnns under heterophily: Are we really making progress? arXiv preprint arXiv:2302.11640 (2023)
3. Rozemberczki, B., Allen, C., Sarkar, R.: Multi-scale attributed node embedding. Journal of Complex Networks **9**(2), cnab014 (2021)
4. Tang, J., Sun, J., Wang, C., Yang, Z.: Social influence analysis in large-scale networks. In: Proceedings of the 15th ACM SIGKDD international conference on Knowledge discovery and data mining. pp. 807–816 (2009)
5. Yang, Z., Cohen, W., Salakhudinov, R.: Revisiting semi-supervised learning with graph embeddings. In: ICML. pp. 40–48 (2016)
